# Supplementary material for: SlideBot: A Multi-Agent Framework for Generating Informative, Reliable, Multi-Modal Presentations
Source: arXiv:2511.09804 source file (2025-11-12)

# Understanding Multi-head Attention

- Multi-head attention enhances model's ability to focus on different parts of input
- It uses multiple attention heads to capture diverse information patterns
- Each head processes input independently and results are concatenated
- Improves performance in sequence modeling tasks like NLP
- Key component in Transformer architectures

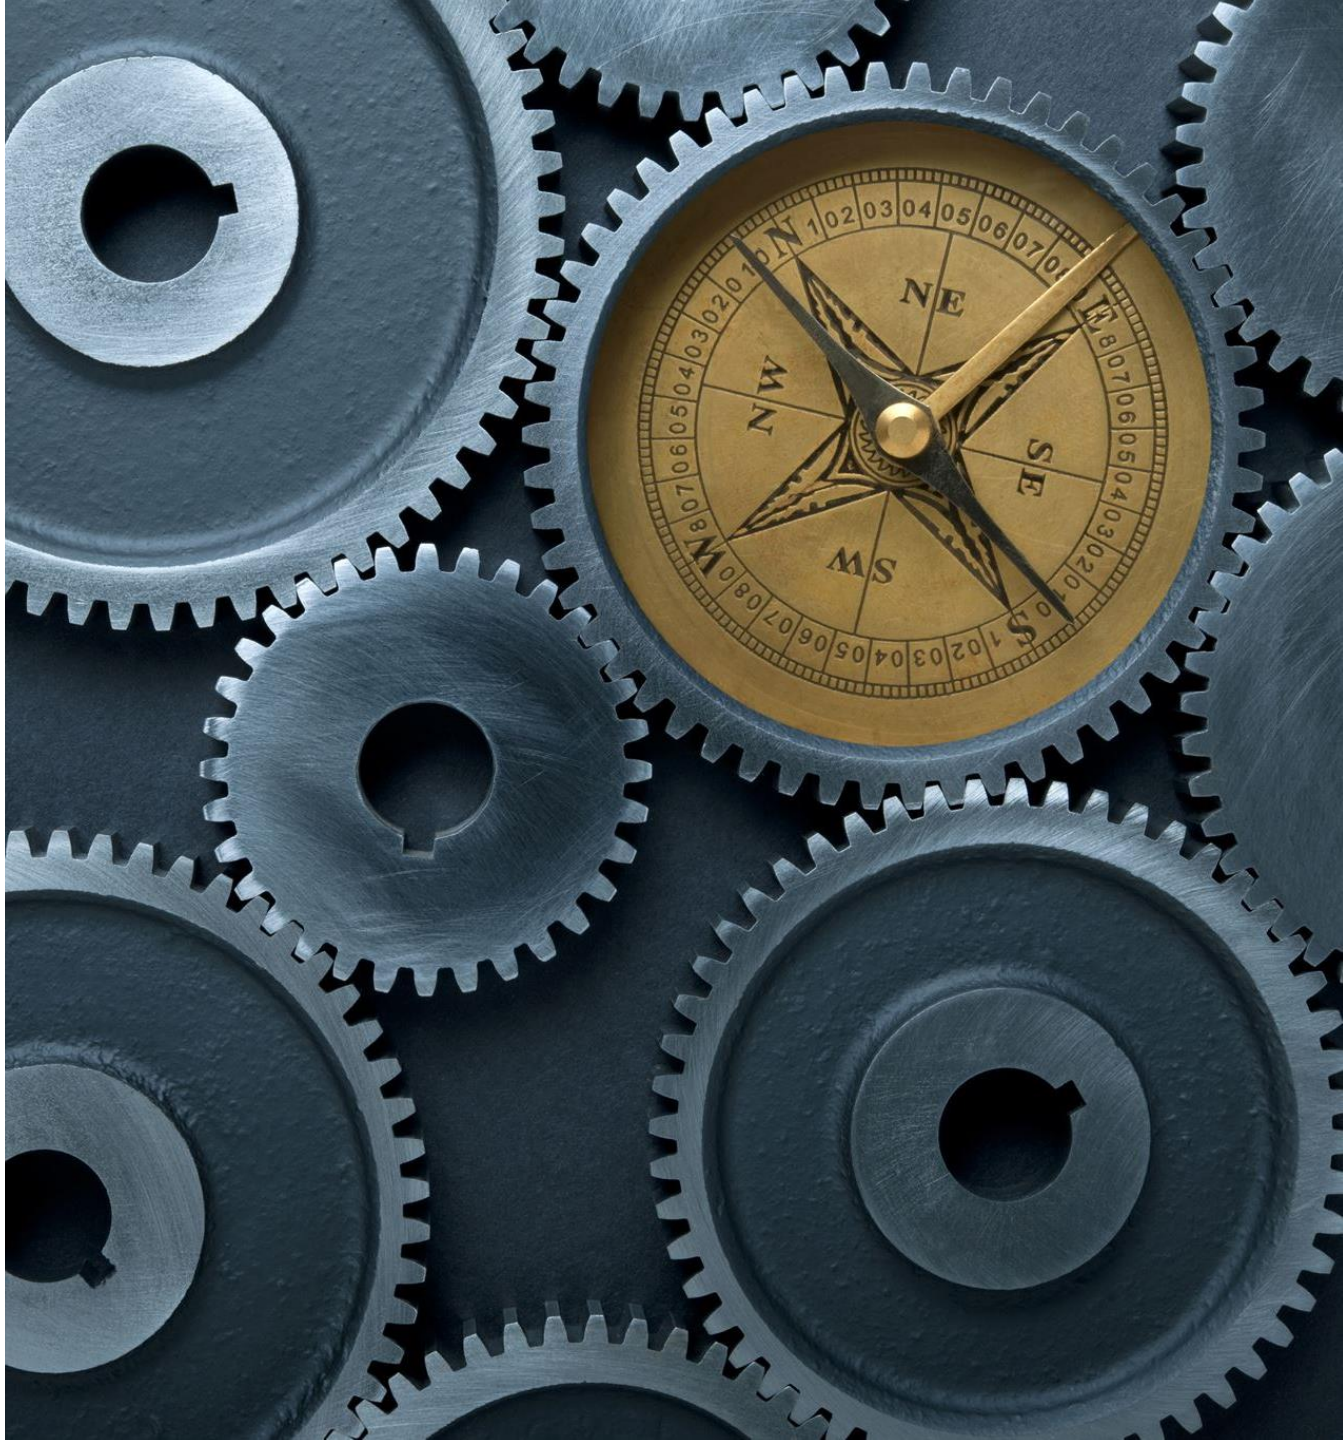

# How Multi-head Attention Works

- Input is projected into queries, keys, and values for each head
- Scaled dot-product attention is computed independently for each head
- Attention weights determine relevance between queries and keys
- Outputs of all heads are concatenated and linearly transformed
- This enables parallel processing and richer feature extraction

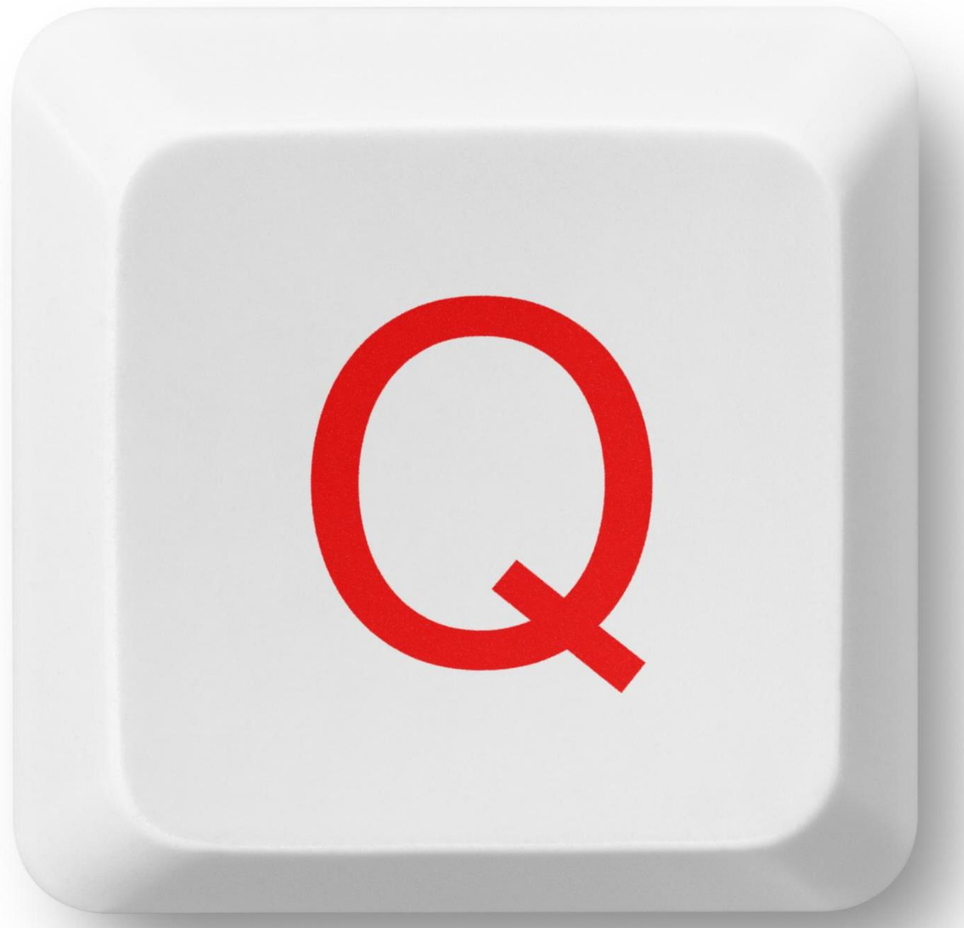

# Mathematical Formulation

- $\text{Attention}(Q,K,V) = \text{softmax}(QK^T / \sqrt{d_k})\, V$
- Multi-head attention applies this attention h times in parallel
- Outputs from each head are concatenated: $\text{concat}(\text{head}_1,\ldots,\text{head}_h)$
- Final output is linear transformation of concatenated heads
- This formulation allows learning diverse representation subspaces

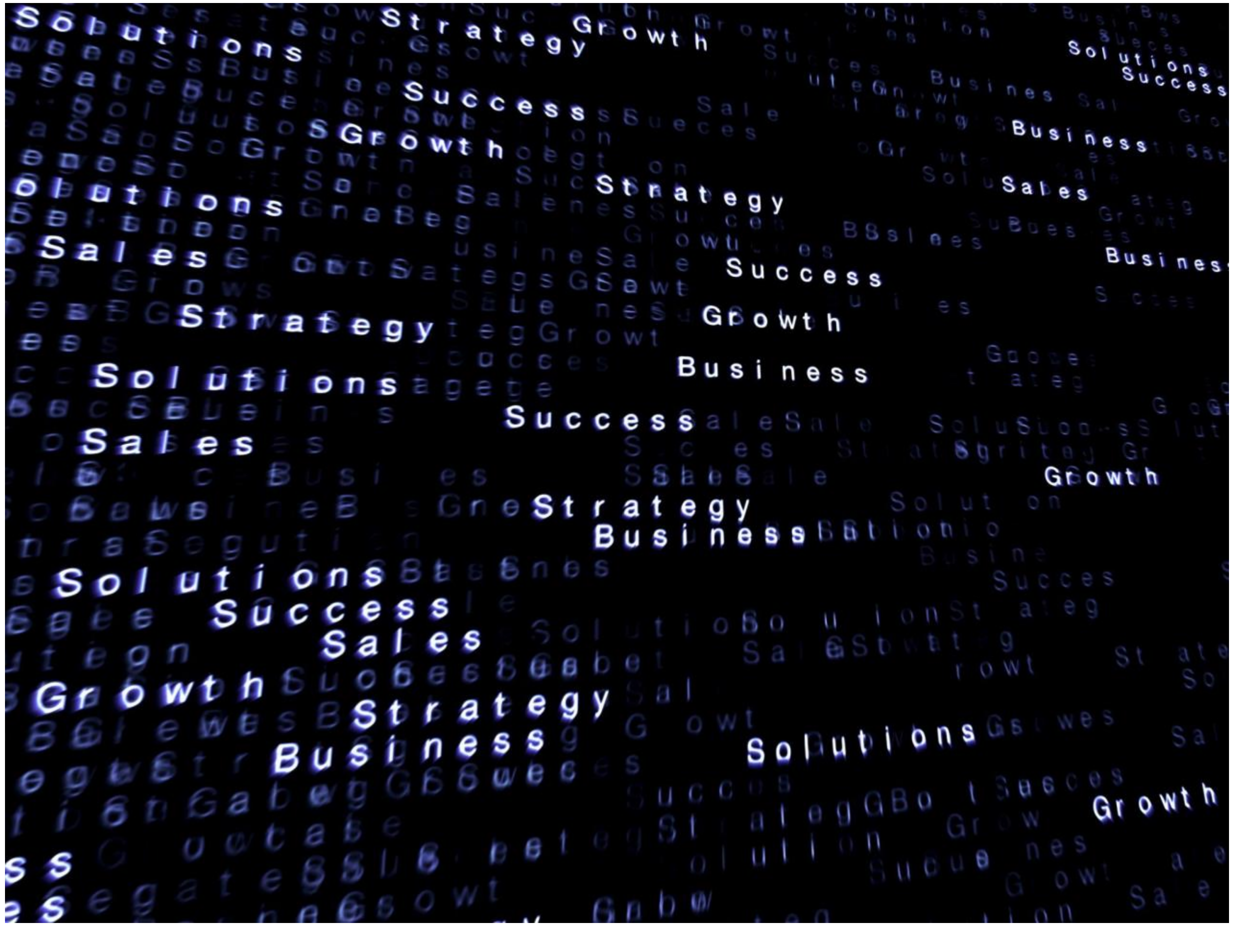

# Advantages of Multi-head Attention

- Captures information from multiple representation subspaces
- Allows the model to focus on different positions simultaneously
- Enhances model's capacity to learn complex patterns
- Improves convergence and generalization in training
- Facilitates parallelization for computational efficiency

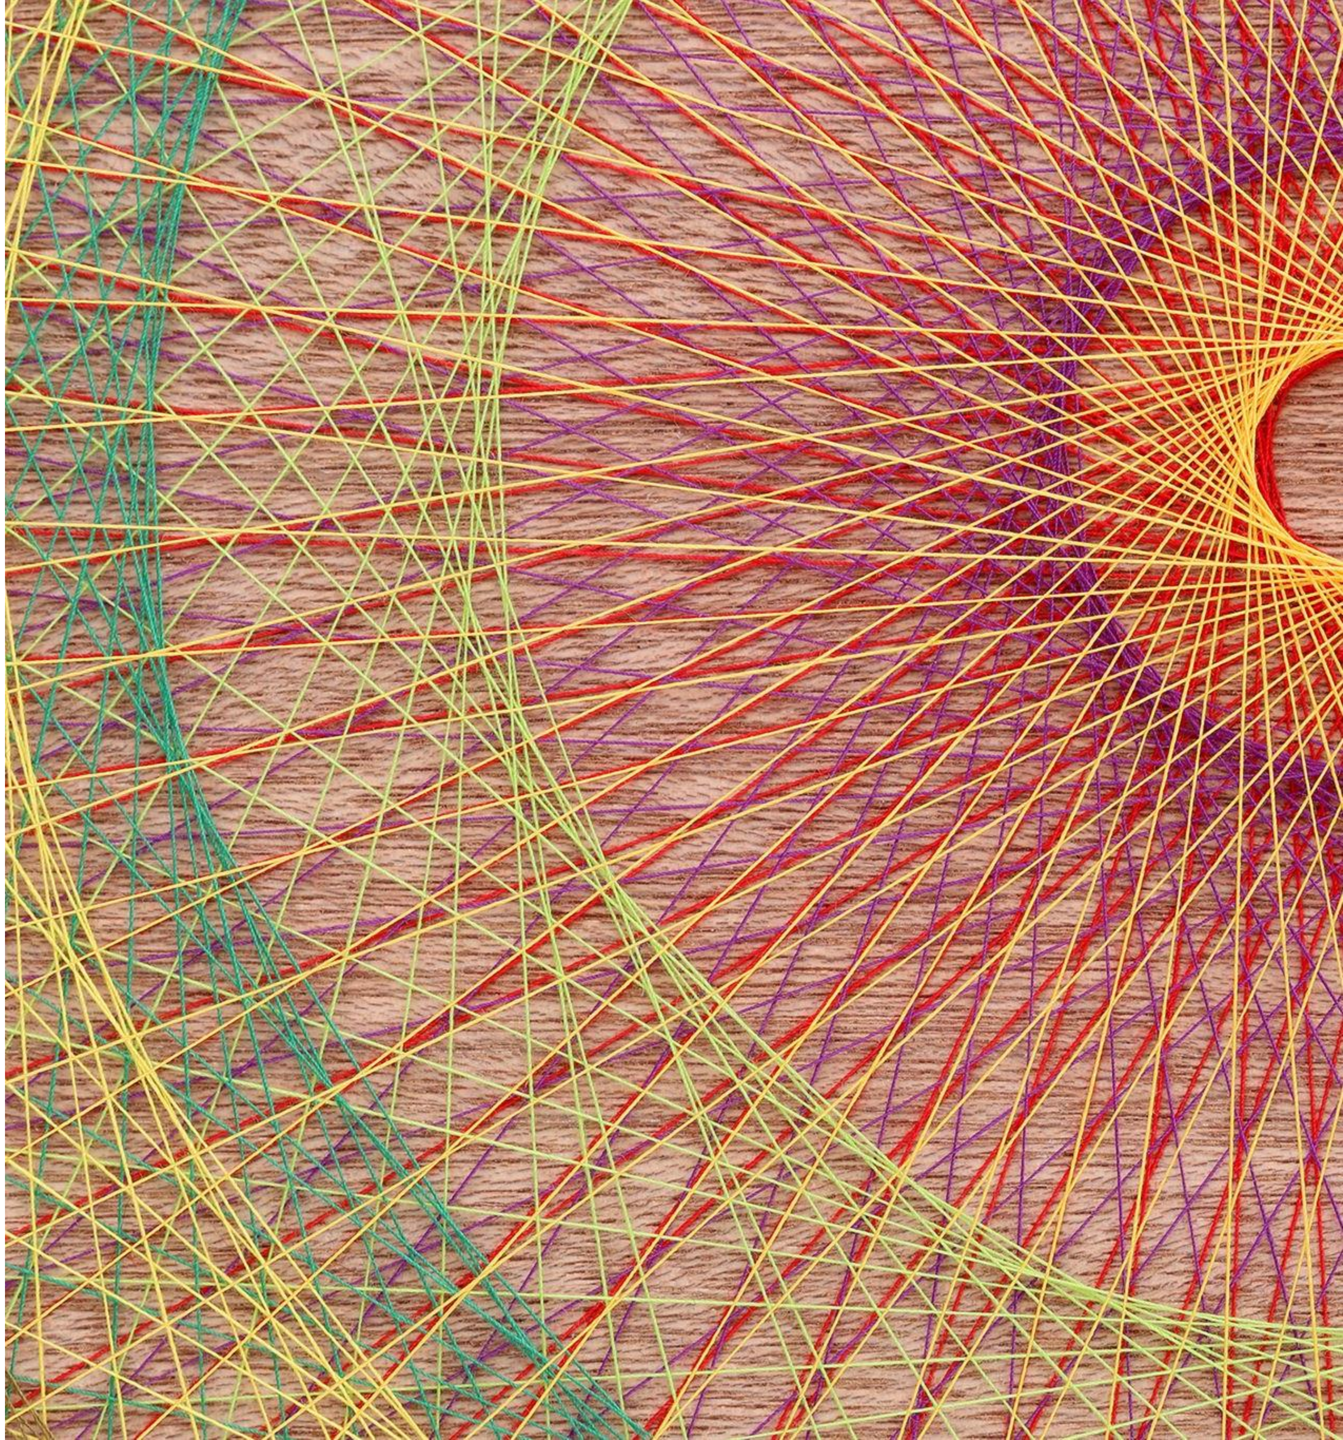

# Applications in Natural Language Processing

- Core component of Transformer models like BERT and GPT
- Improves tasks such as translation, summarization, and question answering
- Enables contextual understanding of words and sentences
- Supports transfer learning with pre-trained models
- Revolutionized NLP state-of-the-art results

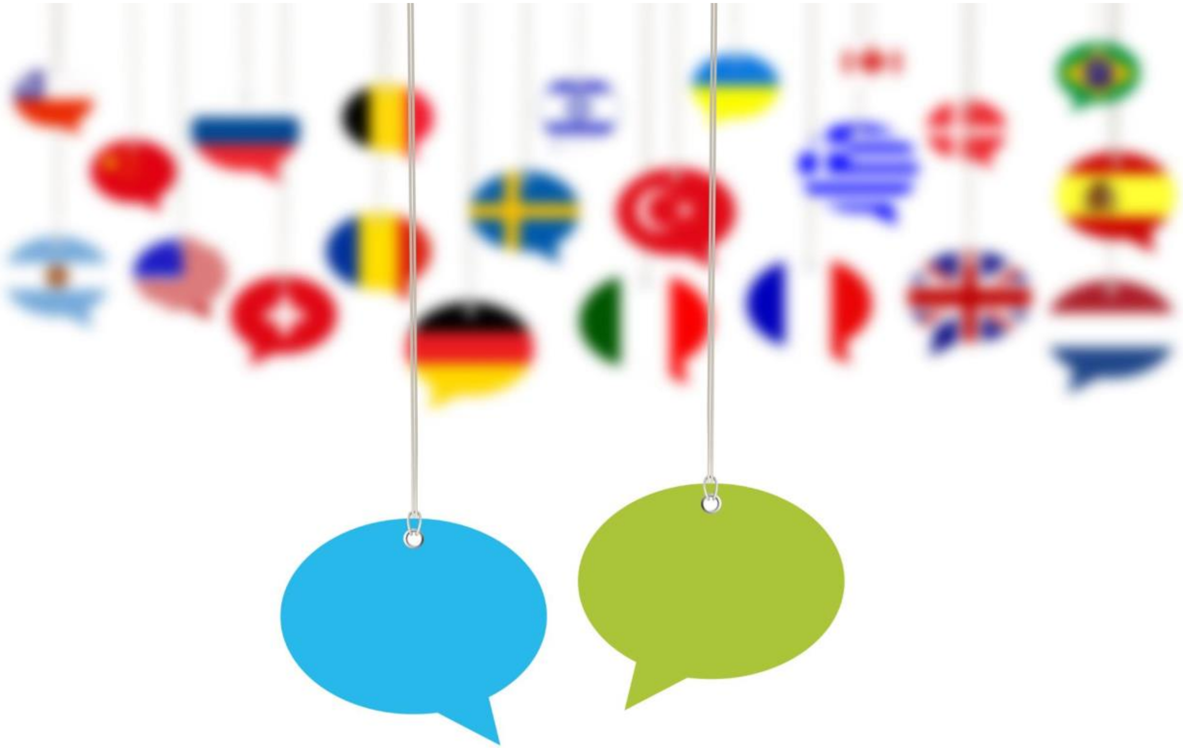

# Challenges and Limitations

- Computational and memory cost increases with number of heads
- Can be sensitive to hyperparameter choices like head count
- May struggle with very long input sequences
- Requires large amounts of training data for optimal performance
- Interpretability of attention weights can be ambiguous

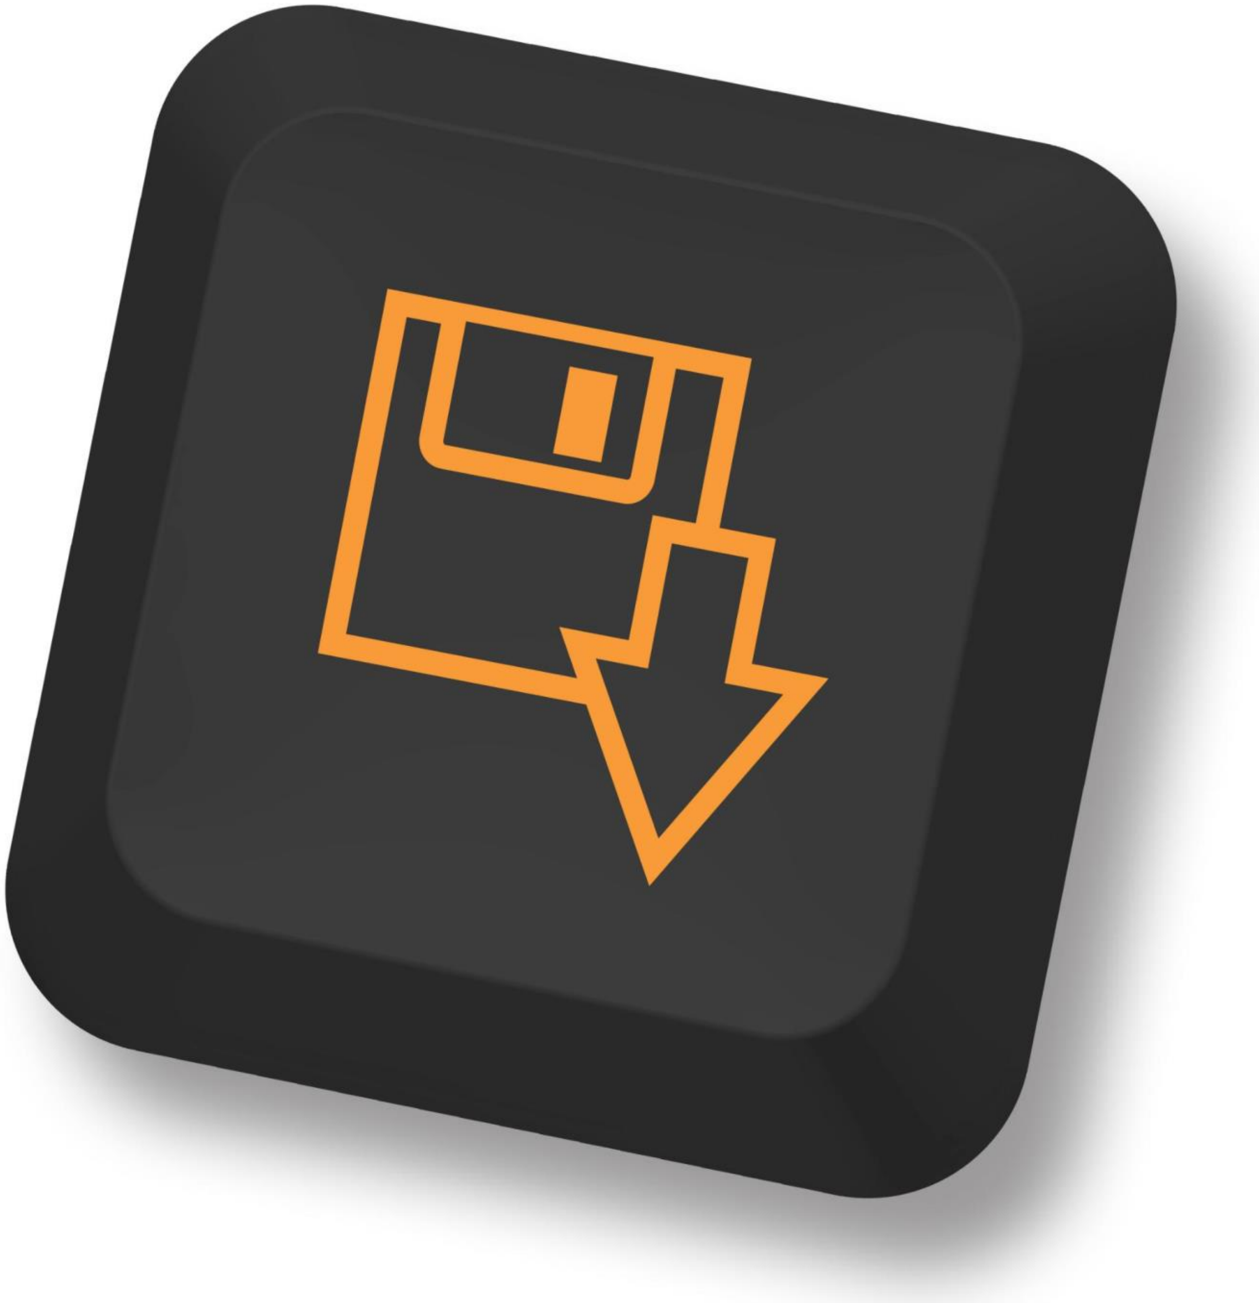

# Future Directions in Attention Mechanisms

- Research into more efficient attention variants
- Integration with other modalities like vision and audio
- Exploration of sparse and adaptive attention models
- Improving interpretability and explainability
- Scaling for extremely large models and datasets

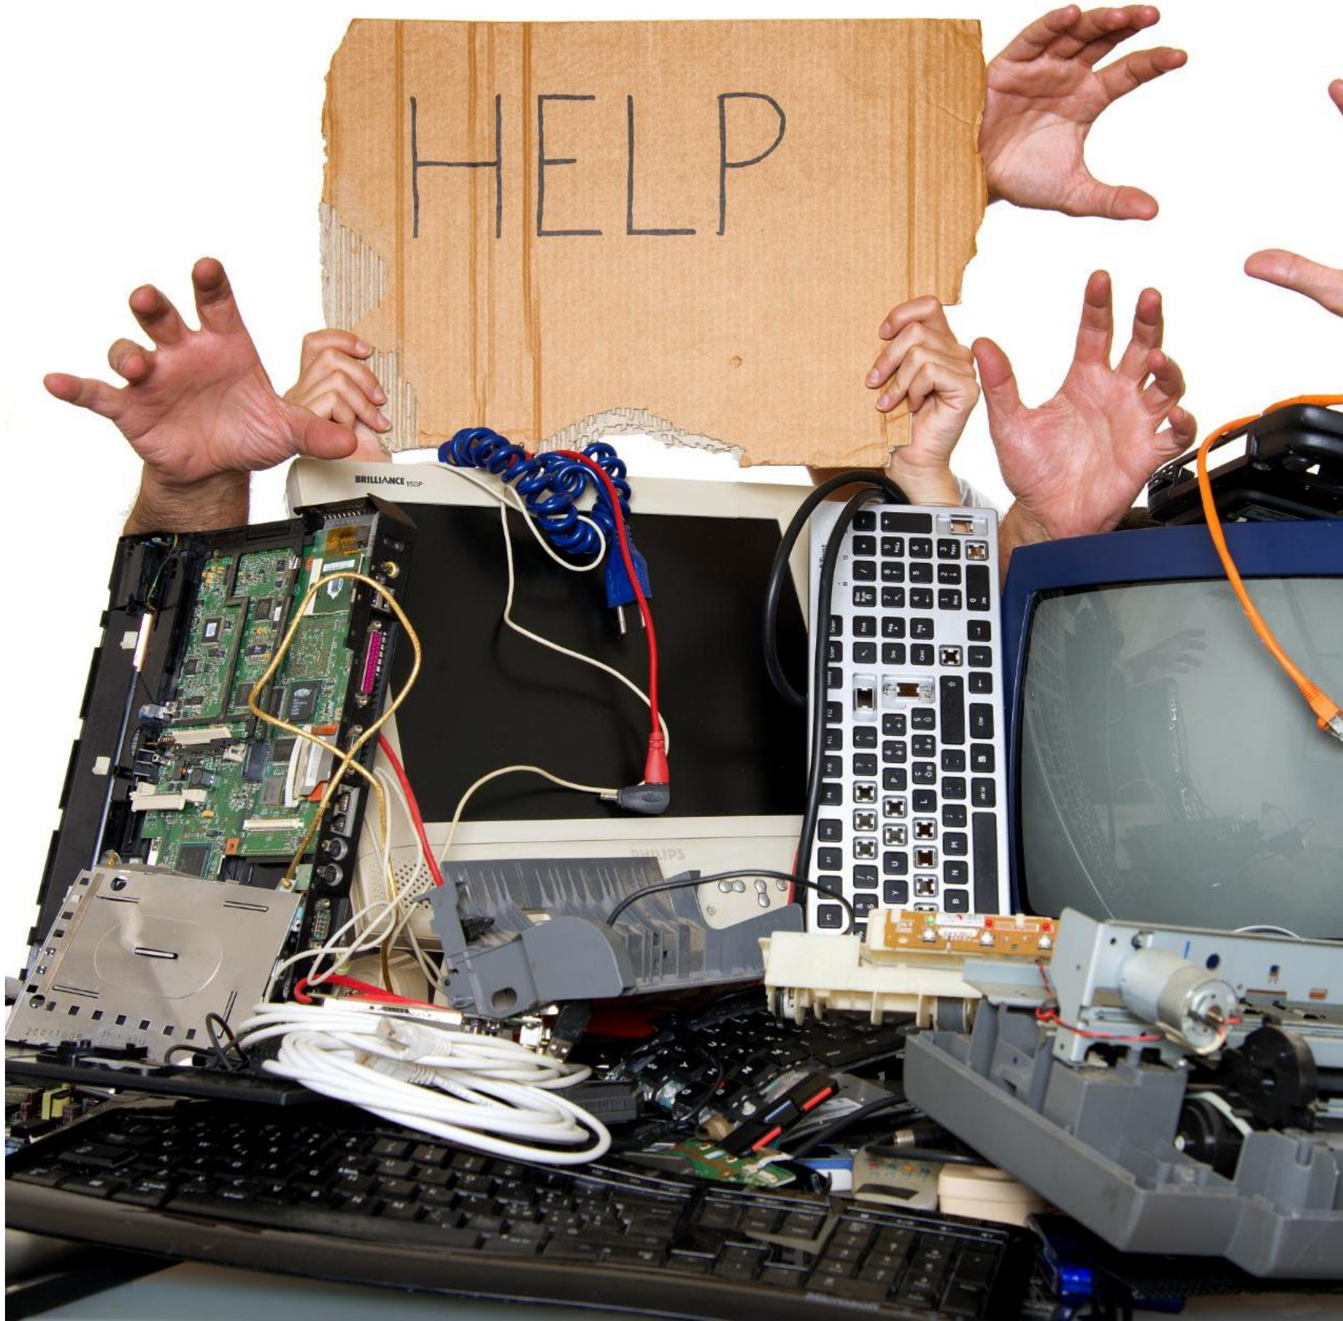

Supplement: Supplementary file 1 [file Copilot_multi-head.pdf]
