# Supplementary material for: SlideBot: A Multi-Agent Framework for Generating Informative, Reliable, Multi-Modal Presentations
Source: arXiv:2511.09804 source file (2025-11-12)
Supplement: Supplementary file 2 [file SlideBot_manifold.pdf]

# Manifold Learning

Your Name

Your Affiliation

2025-08-13

*Generated by SlideBot

# Roadmap

- Introduction
- Importance
- Limitations
- Recent Advancements
- Critical Perspectives
- Future Directions
- Conclusion

# Introduction to the Topic

- **Definition:** Manifold learning focuses on understanding high-dimensional data b[illegible]entifying lower-dimensional structures, or manifolds, within it [1].
- **Dimensionality Reduction:** A key technique in manifold learning that simplifies data while preserving essential features [1].
- **Applications:** Crucial fo[illegible]ltimedia data analysis, including image and audio processing [1].

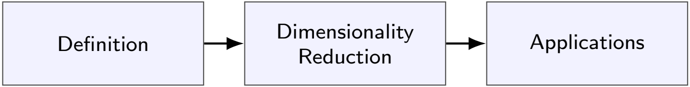

# Why This Topic Matters

- **Complex Data Handling:** Manifold learning effectively manages high-dimensional data complexities, enhancing analysis [1].
- **Multimedia Applications:** Vital for improving performance in image processing, audio analysis, and video recognition [1].
- **Feature Extraction:** Helps in uncovering mean[illegible]ul patterns in complex datasets, leading to better insights [1].

# Motivating Limitations of Early Approaches

- **PCA Limitations:** Principal Component Analysis (PCA) fails to preserve local structures in high-dimensional data [1].
- **High-Dimensional Challenges:** Traditional methods struggle with the curse of dimensionality, leading to suboptimal embeddings [1].
- **Need for Advanced Techniques:** Highlights the necessity for more sophisticated m[illegible]fold learning methods that address these limitations [1].

# Recent Advancements in Manifold Learning

- **Evolution of Techniques:** Recent methods have improved the preservation of local structures in embeddings [1].
- **Diverse Applications:** New algorithms are being applied across various fields, enhancing their utility [1].
- **Focus on Interpretability:** Recent advancements emphas[illegible]ot only performance but also the interpretability of the results [2].

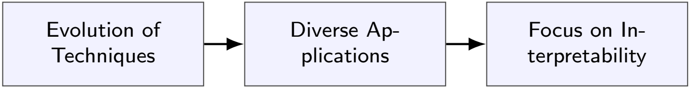

- **Geodesic Distances:** Isomap maintains intrinsic geometry by utilizing geodesic distances [1].
- **Key Formula:**

$$d_{geodesic}(x_i, x_j)$$

- **Preservation of Structure:** Effective[illegible]ptures the manifold structure in high-dimensional data [1].

| | | **Predicted 1** | **Predicted 0** |
|---|---|---|---|
| **Actual** | **1** | TN | FP |
| | **0** | FN | TP |

# Overview of Locally Linear Embedding (LLE)

- **Reconstruction Focus:** LLE reconstructs data points based on their neighbors, preserving local relationships [1].
- **Reconstruction Error Formula:**

$$\text{Reconstruction Error} = \sum_i \|x_i - \sum_{j \in N(i)} w_{ij} x_j\|^2$$

- **Local Structure [illegible]servation:** Enhances the understanding of local data topology [1].

# Overview of t-Distributed Stochastic Neighbor Embedding (t-SNE)

- **Visualization Effectiveness:** t-SNE excels in visualizing high-dimensional data in lower dimensions [1].
- **Cost Function:**

$$C = \sum_i \sum_j p_{ij} \log \frac{p_{ij}}{q_{ij}}$$

- **Divergence Minimization:** Focuses on minimizing divergenc[illegible] between probability distributions for better representation [1].

# Genetic Programming for Manifold Learning

- **Local Topology Preservation:** Introduces a genetic programming approach to enhance local topology preservation [2].
- **Methodology Steps:** Includes initialization, fitness evaluation, selection, and evolution of mappings [2].
- **Impact on Interpretability:** Enhances both p[illegible]rmance and interpretability of manifold learning results [2].

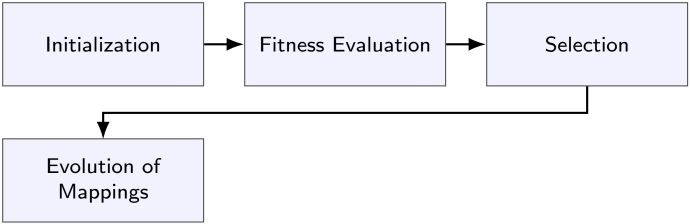

# Results of Genetic Programming Approach

- **Performance Comparison:** Genetic programming outperforms baseline techniques like t-SNE and UMAP [2].
- **Metrics Used:** Improvements quantified through reconstruction error and neighborhood preservation accuracy [2].
- **Practical Implications:** Provides a [illegible]e interpretable framework for understanding complex datasets [2].

# Functorial Manifold Learning

- **Functorial Framework:** Characterizes algorithms as functors mapping pseudometric spaces to optimization objectives [3].
- **Algorithm Hierarchy:** Establishes a hierarchy of algorithms based on their complexity and performance [3].
- **Stability Analysis:** Analyzes stability in the pre[illegible]e of noise, providing insights into algorithm robustness [3].

# Stability Analysis in Functorial Learning

- **Interleaving Distance:** Measures stability of manifold learning algorithms under noise [3].
- **Quantitative Bounds:** Provides bounds on how closely noisy embeddings approximate noiseless ones [3].
- **Practical Relevance:** Crucial [illegible] applications where data imperfections are common [3].

# New Algorithms from Functorial Framework

- **Competitive Performance:** New algorithms derived from the functorial framework show competitive results against existing methods [3].
- **Theoretical Insights:** The framework bridges theoretical concepts with practical advancements in manifold learning [3].
- **Real-World Applicati[illegible]** Demonstrates applicability in various data analysis challenges [3].

# Critical Perspectives

- **Advancements Analysis:** Critical examination of recent advancements in manifold learning [1].
- **Drawbacks:** Discusses potential limitations and areas needing further research [1].
- **Future Research Needs:** I[illegible]tifies gaps in current methodologies that require exploration [1].

# Future Directions

- **Integration of Frameworks:** Explore the integration of new theoretical frameworks into manifold learning [1].
- **Emerging Data Types:** Application of manifold learning methods to new and complex data types [1].
- **Interdisciplinary Approaches:** Encourage c[illegible]boration across fields to enhance manifold learning techniques [1].

# Conclusion

- **Key Takeaways:** Manifold learning is essential for understanding high-dimensional data [1].
- **Applications:** Its applications in multimedia are vast and impactful [1].
- **Future Potentia**[illegible]ontinued advancements will enhance its utility in various fields [1].

# References


Hannes Fassold. A survey of manifold learning and its applications for multimedia. http://arxiv.org/abs/2310.12986v1

Andrew Lensen, Bing Xue, Mengjie Zhang. Genetic Programming for Manifold Learning: Preserving Local Topology. http://arxiv.org/abs/2108.09914v1

Dan Shiebler. Functorial Manifold Learning. http://arxiv.org/abs/2011.07435v6
