# Supplementary material for: SlideBot: A Multi-Agent Framework for Generating Informative, Reliable, Multi-Modal Presentations
Source: arXiv:2511.09804 source file (2025-11-12)
Supplement: Supplementary file 3 [file SlideBot_multi-head.pdf]

# Multi-Head Attention

Your Name

Your Affiliation

2025-07-15

# Roadmap

- Introduction
- Importance
- Limitations
- Recent Advancements
- Critical Perspectives
- Future Directions
- Conclusion

# Introduction to the Topic

- **Attention Mechanisms:** Key [illegible]ponents in machine learning for processing sequential data [1].
- **Sequential Data Processing:** Enhance model performance by focusing on relevant parts of the input [2].
- **Model Performance:** Attention mechanisms improve interpretability and efficiency in various tasks [3].

# Why This Topic Matters

- **Significance in AI:** Attention mechanisms are crucial in natural language processing and computer vision [1].
- **Impact on Interpretability:** They enhance model interpretability, allowing better understanding of decision-making processes [2].
- **Performance Boost:** Attention mechanisms lead to significant improvements in model performance across various applications [3].

# Motivating Limitations of Early Approaches

- **Computational Inefficiency:** Early attention mechanisms struggled with high computational costs, limiting scalability [2].
- **Long-Range Dependencies:** Inability to effectively capture long-range dependencies in data sequences [3].
- **Need for Advancements:** These limitations necessitated the dev[illegible]ment of more sophisticated models like Multi-Head Attention [1].

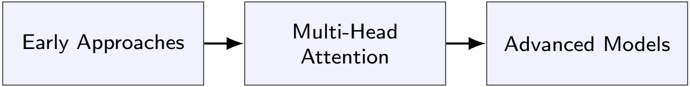

# Recent Advancements - Human Attention Network (HAN)

- **Human Attention Network (HAN):** Introduces a novel architecture that generates human-like attention maps [1].
- **HLAT Dataset Creation:** Developed the Human-Like Attention (HLAT) dataset, enhancing VQA tasks with human-like supervision [1].
- **Empirical Validation:** Demonstrated improv[illegible]ttention accuracy and performance metrics in VQA models [1].

# Contributions of HAN

- **Attention Maps:** Reflect human visual focus, addressing the lack of human attention data in VQA [1].
- **Performance Improvement:** Empirical evidence shows significant enhancements in VQA capabilities through human-like supervision [1].
- **Future Research Direction:** Pave[illegible]e way for more interpretable models in visual understanding [1].

# Methodology of HAN

- **Training Dataset:** The HAN is trained on the VQA-HAT dataset, containing human attention data [1].
- **Supervision Mechanism:** Utilizes a loss function minimizing the difference between model outputs and human-like attention maps [1].
- **Architecture:** Likely employs CN[illegible]r visual inputs and RNNs or transformers for textual inputs [1].

$$L = \frac{1}{N}\sum_{i=1}^{N}(y_i - \hat{y}_i)^2$$

# Results of HAN

- **Attention Accuracy:** VQA models with human-like supervision outperform baseline models significantly [1].
- **Interpretability:** Aligns model attention mechanisms more closely with human visual attention patterns [1].
- **Overall Performance:** Suggests a new di[illegible]ion for enhancing VQA systems through human-like attention [1].

# Recent Advancements - Simulating Hard Attention

- **Soft Attention Mimicking Hard Attention:** Explores how soft attention can replicate hard attention behaviors in transformers [2].
- **Theoretical Framework:** Establishes a connection between hard-attention transformers and language classes defined by linear temporal logic [2].
- **Simulation Techniques:** Introduces unbounded positional embeddings and temperature scaling to enhance soft attention [2].

# Contributions of Hard Attention Simulation

- **Language Classes:** Identifies specific subclasses of languages recognized by hard-attention transformers [2].
- **Unbounded Positional Embeddings:** Allows soft-attention transformers to focus on specific input positions effectively [2].
- **Temperature Scaling:** Adjusts the softmax function t[illegible]arpen focus on relevant inputs, mimicking hard attention [2].

# Methodology of Hard Attention Simulation

- **Mathematical Formulation:** Defines the softmax function with temperature scaling to simulate hard attention [2].
- **Attention Score Distribution:** Adjusts temperature based on the minimum gap between attention scores [2].
- **Empirical Evidence:** Demonstrates that soft-attention transformers can achieve similar performance levels to hard-attention models [2].

$$\text{softmax}(x_i) = \frac{e^{x_i/T}}{\sum_j e^{x_j/T}}$$

# Results of Hard Attention Simulation

- **Performance Levels:** Soft-attention transformers replicate hard-attention behaviors effectively under certain conditions [2].
- **Flexibility:** Highlights the adaptability of soft attention to behave like hard attention when necessary [2].
- **Implications for Model Design:** Insi[illegible] could enhance future model designs in NLP and beyond [2].

# Recent Advancements - Agent Attention

- **Agent Attention Mechanism:** Introduces a new attention mechanism that improves efficiency in transformers [3].
- **Agent Tokens:** Incorporates a smaller set of agent tokens for information aggregation and broadcasting [3].
- **Computational Efficiency:** Ach[illegible]s a balance between efficiency and global context modeling [3].

# Contributions of Agent Attention

- **Integration of Agent Tokens:** Enhances computational efficiency while maintaining expressiveness [3].
- **Reduced Computational Costs:** Designed with fewer agent tokens, beneficial for high-resolution tasks [3].
- **Generalized Linear Attention:** Establishes equivalenc[illegible] linear attention, leveraging strengths of both mechanisms [3].

# Methodology of Agent Attention

- **Attention Mechanism Definition:** Defined as a quadruple $(Q, A, K, V)$, where $A$ aggregates information from $K$ and $V$ [3].
- **Information Aggregation:** Agent tokens aggregate information based on queries, enhancing global context access [3].
- **Mathematical Interaction:** Provides a formul[illegible]n demonstrating efficient computation through agent tokens [3].

---

**Input:** Query $Q$, Agent $A$, Key $K$, Value $V$
**Output:** Output $O$

$O \leftarrow A(K, V)$
**return** $O$

---

# Results of Agent Attention

- **Performance Improvements:** Agent Attention outperforms traditional Softmax attention in various vision tasks [3].
- **High-Resolution Tasks:** Particularly effective in high-resolution scenarios, enhancing speed and accuracy [3].
- **Practical Implications:** Accelerates image genera[illegible] processes while improving quality without extra training [3].

# Critical Perspectives

- **Limitations of Advancements:** Address potential shortcomings in the proposed attention mechanisms [2].
- **Areas for Improvement:** Identify gaps in current methodologies and suggest enhancements [3].
- **Future Research Needs:** Emphasize th[illegible]cessity for ongoing exploration in attention mechanisms [1].

# Future Directions

- **Hybrid Models:** Explore the integration of different attention mechanisms for improved performance [3].
- **Efficiency Enhancements:** Focus on further reducing computational costs while maintaining effectiveness [2].
- **Interpretability Improvements:** Investigat[illegible]ethods to enhance the interpretability of attention mechanisms [1].

# Conclusion

- **Key Takeaways:** Advancements in attention mechanisms are crucial for future AI applications [3].
- **Impact on Model Design:** These developments enhance model interpretability and performance [2].
- **Future Implications:** Continued research in at[illegible]ion mechanisms will shape the landscape of AI technologies [1].

# References

Qiao, T., Dong, J., & Xu, D. (2017). Exploring Human-like Attention Supervision in Visual Question Answering. http://arxiv.org/abs/1709.06308v1

Yang, A., Strobl, L., Chiang, D., & Angluin, D. (2024). Simulating Hard Attention Using Soft Attention. http://arxiv.org/abs/2412.09925v2

Han, D., Ye, T., Han, Y., Xia, Z., Pan, S., Wan, P., Song, S., & Huang, G. (2023). Agent Attention: On the Integration of Softmax and Linear Attention. http://arxiv.org/abs/2312.08874v3
