# Supplementary material for: SlideBot: A Multi-Agent Framework for Generating Informative, Reliable, Multi-Modal Presentations
Source: arXiv:2511.09804 source file (2025-11-12)
Supplement: Supplementary file 4 [file Zero_neurotransmitters.pdf]

# Neurotransmitters

Your Name

Your Institution

January 7, 2025

# Roadmap

Introduction

Types of Neurotransmitters

Mechanism of Action

Major Neurotransmitters

Neurotransmitter Imbalance and Disorders

Conclusion

References

# Introduction

- Definition of neurotransmitters
- Importance in the nervous system
- Overview of types of neurotransmitters

# Types of Neurotransmitters

- Excitatory neurotransmitters
- Inhibitory neurotransmitters
- Modulatory neurotransmitters

# Mechanism of Action

- Synthesis and storage
- Release and receptor binding
- Termination of action

# Major Neurotransmitters

- Acetylcholine
- Dopamine
- Serotonin
- GABA
- Glutamate

# Neurotransmitter Imbalance and Disorders

- Depression
- Schizophrenia
- Parkinson's disease
- Alzheimer's disease

# Conclusion

- Summary of key points
- Importance of neurotransmitter research
- Future directions

# References

Purves, D., Augustine, G. J., Fitzpatrick, D., Hall, W. C., LaMantia, A.-S., White, L. E. (2018). *Neuroscience* (6th ed.). Sinauer Associates.

Kandel, E. R., Schwartz, J. H., Jessell, T. M., Siegelbaum, S. A., Hudspeth, A. J. (2013). *Principles of Neural Science* (5th ed.). McGraw-Hill.

Bear, M. F., Connors, B. W., Paradiso, M. A. (2015). *Neuroscience: Exploring the Brain* (4th ed.). Wolters Kluwer.
